# Supplementary material for: A Checks-and-Balances Framework for Context-Aware Ethical AI Alignment
Source: arXiv:2502.00136 source file (2025-05-28)
Supplement: Supplementary file 2 [file AppendixBEAMInterpretation.tex]

\section{BEAM Spectra Interpretation}

\begin{enumerate}
\item First row: This spectrum is particularly insightful for discussions in psychology, education, leadership, and moral philosophy. It illustrates how individuals might transition from states of intense fear to actions characterized by great moral and physical courage. Each step represents a stage in emotional development or response to challenging situations, offering a framework for understanding how people can rise above their fears to perform acts of significant bravery and altruism.

Overall, this spectrum not only portrays a journey through varying degrees of fear and courage but also encapsulates the transformative potential within individuals to act heroically in the face of adversity.

\item Second row: This emotional spectrum elegantly illustrates how emotions can transition from profound sorrow to extreme happiness. It is particularly relevant in psychological studies, therapeutic contexts, and philosophical discussions about the range and nature of human emotions. Each emotional state on this spectrum offers insight into how individuals might process and recover from sadness, ultimately finding joy and possibly reaching ecstatic experiences. This spectrum can serve as a framework for understanding emotional resilience and the potential for emotional transformation and growth.

\item Third row:
This spectrum beautifully illustrates the journey from initial suspicion and caution through acceptance and respect, culminating in deep trust and admiration. It's particularly relevant in contexts where trust building and social cohesion are critical, such as in leadership, team dynamics, community relations, and personal relationships. Each stage reflects a deeper layer of positive engagement and emotional commitment, providing insights into how relationships can evolve and strengthen over time. This framework can serve as a guide for understanding and developing strategies for fostering trust and admiration in various social and professional settings.

\item Fourth row: This spectrum effectively maps out how an individual can transition from passive disengagement (negligence, indifference, apathy) through a state of balanced caution to active and engaged states (interest, anticipation, vigilance). It offers insights into the psychological journey from inaction through moderate engagement to intense proactive involvement. This framework is particularly relevant in contexts that require understanding and managing risk, such as safety protocols, healthcare, education, and personal growth initiatives, as it highlights how attitudes toward responsibility and awareness can evolve and improve.

\item Fifth row: This spectrum is particularly useful for understanding emotional management and conflict resolution strategies, as it depicts the gradient from intense emotional disturbance through to complete serenity. It can be applied in various fields, including psychology, conflict resolution, stress management, and even in designing environments or experiences that aim to reduce stress and promote peace.

Overall, this emotional spectrum effectively portrays a journey from the depths of aggressive negativity to the pinnacle of peaceful positivity, offering a valuable framework for discussing and exploring emotional states and transformations.

\item Sixth row: This spectrum effectively maps a journey from profound negative feelings of loathing and disgust, through a state of neutrality (indifference), to the positive emotions of interest, anticipation, and culminating in enthusiasm. It's particularly useful for understanding emotional responses in various contexts, such as consumer behavior, audience engagement, and personal relationships. Each stage reflects a distinct level of emotional engagement, providing a framework for understanding how emotional states can evolve and impact behavior and decision-making.
\end{enumerate}
