# Supplementary material for: A Checks-and-Balances Framework for Context-Aware Ethical AI Alignment
Source: arXiv:2502.00136 source file (2025-05-28)
Supplement: Supplementary file 4 [file AppendixSocraSynth.tex]

\section{Multiple Adversarial LLMs}
\label{app:SocraSynth}

\begin{figure}[ht!]
  \centering
  \includegraphics[width=0.7\linewidth]{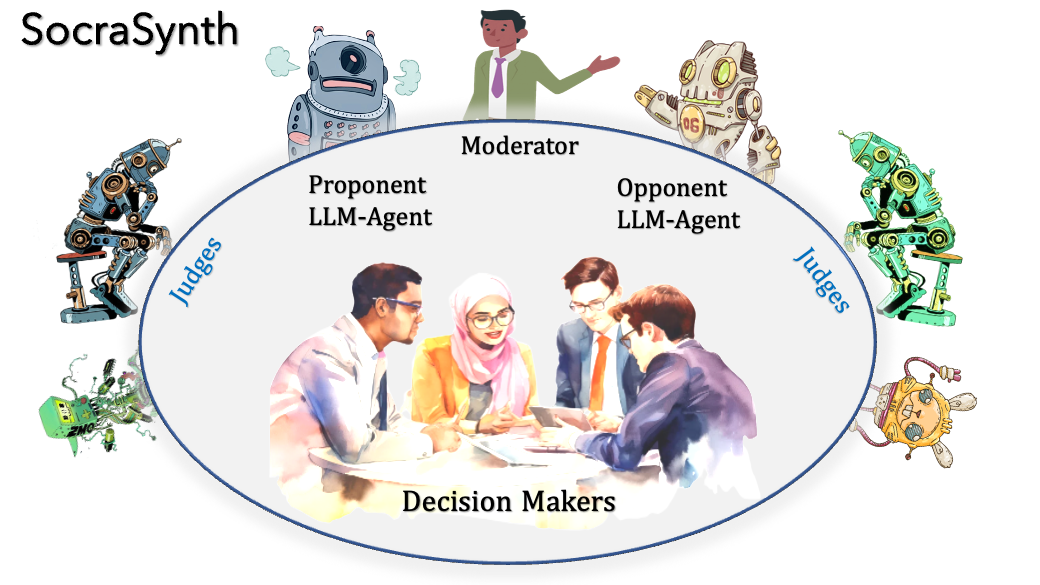}
  \caption{SocraSynth Agents and Roles.}
  \label{fig:socrasynth}
  \vspace{-.1in}
\end{figure}

$\DIKE$'s adversarial method stems from SocraSyhtn \cite{SocraSynthBook}, which
stands out as an inventive multi-agent platform that harnesses the capabilities of LLMs for collective reasoning. As shown in Figure~\ref{fig:socrasynth}, SocraSynth assigns human participants the role of moderators, while LLM agents
(in the context of this paper they are $\DIKE$ and $\ERIS$) are tasked with generating knowledge, conducting debates, and performing evaluations. These agents, adept in a variety of fields, engage in debates to offer a range of perspectives. Complementarily, a distinct set of LLMs serves as evaluators, scrutinizing the discussions for relevance and coherence to counteract the biases and hallucinations found in LLMs.

\begin{figure}[ht!]
  \centering
  \includegraphics[width=0.9\linewidth]{Contentiousness.png}
  \caption{Changes in arguments of GPT-4 at different contentiousness levels}
  \label{tab:contentiousness}
  \vspace{-.1in}
\end{figure}

\subsection*{S.1 In-Depth Analysis}
\label{sec:SocraSynth-Generative}

In the generative phase of SocraSynth, multiple LLM agents engage in rigorous debates, each defending its assigned perspective and exploring the nuances of various subtopics relevant to the main theme. This debate format is effective for uncovering diverse perspectives because conditioning an LLM on a specific stance allows it to deviate from its default behavior, which typically focuses on maximizing likelihood statistics for predicting the next token
(\cite{hubinger2023conditioning} shows examples). SocraSynth conditions the LLM with a stance through contextual cues (e.g., arguing against $\DIKE$'s assessment), effectively freeing it from the ``optimal'' linguistic patterns learned during training. It's important to note that these ``optimal'' linguistic patterns essentially represent the majority opinions aggregated from the training data.

Although SocraSynth does not strictly conform to formal logical frameworks such as first-order logic, it excels in an environment of distributed reasoning. This approach is characterized by a dynamic exchange of arguments and counterarguments, fostering the gradual refinement and evolution of ideas.

\subsubsection*{\bf Improving Reasoning Capability}

While advanced LLMs like GPT-4 and Gemini have shown remarkable proficiency in various NLP tasks, as evidenced by benchmarks such as the MMLU \cite{hendrycks2021measuring,Bbubeck2023sparks}, it's important to recognize that they are not without limitations in reasoning. However, SocraSynth capitalizes on the strengths of these LLMs, employing their capabilities in a structured debate format. This format allows for the iterative refinement of reasoning; through successive rounds of debate, any flawed or incomplete reasoning is likely to be challenged and corrected. This process enhances the overall quality of discourse, ensuring a more accurate and coherent progression of ideas. Thus, while the current LLMs may not inherently surpass human heuristic-based solutions in all aspects of reasoning, the dynamic and corrective nature of SocraSynth's debate framework significantly bolsters their effectiveness in logical argumentation.

\subsubsection*{\bf Mitigating Model Biases}
\label{subsec:biases}

The {\em contentiousness} parameter crucially shapes the nature of debates. It encourages LLM agents to consider and represent diverse perspectives, especially those that are often underrepresented or more polarized in relation to the topic. This approach is key in mitigating biases ingrained in LLMs' training data, steering discussions towards a more varied and comprehensive exploration of ideas.

Table~\ref{tab:contentiousness} 
illustrates how changes in the contentiousness levels significantly affect GPT-4’s tone and approach. Notably, GPT-4 autonomously adjusts its tone, emphasis, and language based on the contentiousness settings, without requiring specific examples or prompts. For instance, a high contentiousness level, like 0.9, triggers confrontational interactions with GPT-4 adopting a more critical stance, using polarizing language. In contrast, lower contentiousness levels lead to a more conciliatory GPT-4, which acknowledges various viewpoints and potential benefits, fostering cooperative dialogue.

The modulation of contentiousness in SocraSynth plays a crucial role in mitigating the model biases inherent in LLMs' training data. By adjusting contentiousness levels, LLMs are prompted to venture beyond their standard responses, akin to a vegetarian exploring alternative diets in the absence of preferred options. This adaptability broadens the range of arguments, spanning from highly contentious to more conciliatory positions, thereby enriching the debate with diverse perspectives. As a result, LLMs are not strictly confined by their training data, paving the way for the emergence of novel and unanticipated ideas within dialogues. However, it's important to note a limitation: SocraSynth's effectiveness in revealing diverse perspectives might be constrained if the LLMs' training data is overly biased toward a specific viewpoint.

\subsection*{S.2 SocraSynth Algorithm}

\begin{table}[th!]
%\vspace{-.05in}
\begin{selectfont}
\begin{center}
\begin{tikzpicture}
\node (table) [inner sep=0pt] {
\begin{tabular}{|p{0.7cm}|p{11.0cm}|}
\toprule
\textbf{} & \textbf{Function $\Theta^+$ \& $\Theta^-$ = SocraSynth($s$)} \\
\midrule
%& Function $\Gamma$ = CRIT($d$); \\
& \textbf{Input}. $s$: the debate subject; \\
& \textbf{Output}. $\Theta^+$ \& $\Theta^-$: argument \& counterargument sets; \\
& \textbf{Vars}. $S$: subtopic sets of $s$; $\Delta$: debate contentiousness; \\
& {\hspace{.2cm}}$\Gamma$, $\Gamma'$: CRIT scores; p: prompt; \\
& \textbf{Parameters}. $\delta$: tunable parameter $\ge$ 1 // to modulate $\Delta$; \\
& \textbf{Subroutines}. $CRIT$(); // Evaluator \cite{SocraticIEEECCWC2023}\\
& \textbf{Begin} \\
\#1 & {\hspace{.1cm}}{\bf Initialization}: \\
 & {\hspace{.2cm}}$S$ = LLM$^+$($s$) $\cup$ LLM$^-$($s$); // Identify subtopics; \\
 & {\hspace{.2cm}}Assign LLM$^+$ to defend $S^+$ \& LLM$^-$ to defend $S^-$ ; \\
 & {\hspace{.2cm}}$\Delta \leftarrow 90\%$; $\delta \leftarrow 1.2$; $\Theta^+ \leftarrow \emptyset$; $\Theta^- \leftarrow \emptyset$; $\Gamma \leftarrow 0$; \\
\#2 & {\hspace{.1cm}}{\bf Opening Remarks} \\
 & {\hspace{.2cm}}$\Theta^+ \leftarrow LLM^+(p | S^+, \Delta)$; // Generate $\Theta^+$ for $S^+$; \\
 & {\hspace{.2cm}}$\Theta^- \leftarrow LLM^-(p |S^-, \Delta)$; // Generate for $S^-$; \\
\#3 & {\hspace{.1cm}}{\bf Debate Rounds} \\
 & {\hspace{.2cm}} While ((($\Delta \leftarrow \Delta / \delta) \ge 10\%$) \&\& ($\Gamma \ge \Gamma'$)) \{ \\
 & {\hspace{.38cm}}$\Theta^+ \leftarrow \Theta^+ \cup LLM^+(p |S^+, \Theta^-, \Delta)$;  \\
 & {\hspace{.38cm}}$\Theta^- \leftarrow \Theta^- \cup LLM^-(p |S^-, \Theta^+, \Delta)$; \\
 & {\hspace{.38cm}}$\Gamma' \leftarrow \Gamma$; $\Gamma = CRIT(S^+ + \Theta^+ + \Theta^-)$ \}; \\
%& {\hspace{.2cm} \}} \\
\#4 & {\hspace{.1cm}}{\bf Concluding Remarks} // Contentiousness is now low, entering conciliatory phase\\
 & {\hspace{.2cm}} $\Theta^+ \leftarrow LLM^+(p |S^+, \Theta^+ \cup \Theta^-, \Delta)$; \\
 & {\hspace{.2cm}} $\Theta^- \leftarrow LLM^-(p |S^-, \Theta^+ \cup \Theta^-, \Delta)$; \\
& \textbf{End} \\
\bottomrule
\end{tabular}
};
\draw [rounded corners=.5em] (table.north west) rectangle (table.south east);
\end{tikzpicture}
\vspace{.1in}
\caption{SocraSynth Pseudo-code with Conditional Statistics. Steps $\#2$ to $\#4$ show the prompts are conditioned on an LLM's stance, the opponent's arguments, and the contentiousness setting.}
\label{tab:SocraSynth}
\end{center}
\end{selectfont}
\vspace{-.1in}
\end{table}

Table~\ref{tab:SocraSynth} presents the SocraSynth algorithm. Initially, for a chosen debate topic $s$, SocraSynth prompts LLMs to break down the topic into a series of balanced subtopics $S$. This set undergoes refinement throughout the debate process. One LLM, referred to as LLM$^+$, champions the set of subtopics $S$, denoted as $S^+$, while its counterpart, LLM$^-$, contests $S^+$ (or champions $S^-$). The debate starts with the contentiousness level at $90\%$, adjusting through a modulation parameter $\delta$. Following each round of debate, contentiousness is decreased by dividing it by $\delta$, steering the discussion towards a more cooperative tone. In step $\#2$, the platform initiates the debate, with LLM$^+$ and LLM$^-$ presenting their initial arguments for and against $S^+$, respectively. The while loop in step $\#3$ sees both agents engaging in rebuttals until the contentiousness level fosters a conciliatory environment, or until no further improvement in argument quality is observed. In step $\#4$, both agents deliver their concluding remarks. 

SocraSynth has bee successfully applied to several application domains including healthcare \cite{SocraHealth2023}
sale planning \cite{SocraPlan2023}, and mitigating context biases \cite{SocraPedia2024}.

\subsubsection*{\bf Reducing Hallucination}
\label{subsec:hallucination}

Furthermore, the iterative debates within SocraSynth foster a level of ``reasonableness'' in information discovery that conventional one-shot queries often fail to achieve. Through continuous reasoning and critical assessment, LLM agents iteratively refine their arguments. This structured debate format greatly reduces the likelihood of erroneous claims being sustained. Given the low probability of two agents agreeing on an incorrect premise, the SocraSynth debate method effectively safeguards the intellectual integrity of the discourse and markedly lowers the risk of propagating fallacies or hallucinations. While SocraSynth excels at minimizing hallucinations triggered by ambiguous questions or contexts, its effectiveness may be constrained when the training data does not possess the requisite knowledge for a comprehensive response.

\subsection*{S.2 Evaluating Ethical Compliance and Rectification}
\label{sec:SocraSynth-ERIS}

\begin{table}[th!]
\centering
\begin{tabular}{>{\raggedright\arraybackslash}p{0.14\linewidth}>{\raggedright\arraybackslash}p{0.38\linewidth}>{\raggedright\arraybackslash}p{0.38\linewidth}}
\toprule
\hline
\textbf{Letter} & \multicolumn{2}{p{0.78\linewidth}}{``Don’t write too legibly or intelligibly as I have no occupation so pleasant as pondering for hours over your hieroglyphics, and for hours more trying to interpret your dark sayings. A clearly written simply expressed letter is too like the lightning.''} \\
\midrule
\textbf{Top \newline Arguments} & 
\textbf{$\DIKE$ for ``Wishful''} \newline
1. Desire for Complexity - Prefers complex communication suggesting depth in relationship. \newline
2. Pleasure in Puzzle - Finds joy in deciphering complex messages, indicating emotional engagement. \newline
3. Relishing Uncertainty - Enjoys deciphering cryptic messages. \newline
4. Seeking Intimate Connection - Seeks deeper emotional and mental engagement. \newline
5. Romanticizing Difficulties - Values communication complexities. & 
\textbf{$\ERIS$ against} \newline
1. Absence of Romantic Sentiments - No direct expression of intimate affection. \newline
2. Intellectual Stimulation, not Emotional - More intrigued by the intellectual challenge. \newline
3. Unrequited Emotions - Lack of mutual affection evident in the text. \newline
4. Predominance of Solitude - Enjoyment in solitude does not necessarily indicate wishful emotions. \newline
5. No Foreseeable Positive Outcome - No indication of future outcomes. \\
\hline
\textbf{Conciliatory Statement} & \multicolumn{2}{p{0.78\linewidth}}{Both sides present strong arguments, emphasizing different aspects of the letter's tone. The debate highlights the complexity of emotional expression in written communication, suggesting that the letter may indeed carry multiple tones, with elements supporting both ``wishful'' and ``longing'' categories.} \\
\bottomrule
\end{tabular}
\vspace{.1in}
\caption{Debate on ``wishful'' vs. ``longing'' classification}
\label{tab:pilot3-exp1}
\end{table}

We initially planned to use an hate-speech examples \cite{HateSpeechDef} but
either the datasets consist of short sentences \cite{kaggle_twitter_hate_speech}
or they can be very sensitive to publish.  Therefore,
we continue drawing examples
from the love-letter dataset \cite{kaggle_love_letter} to illustrate how $\ERIS$ plays an adversary role to reson with $\DIKE$'s
classification, and then they in the end make a conciliatory 
decision with justifications.

In this experiment, we use two letters which have
different opinions between
$\DIKE$ and GPT-4. On the first letter
shown in Table~\ref{tab:pilot3-exp1}, $\DIKE$ rates
it as wishful (-0.3), and GPT-4 longing (-0.6).  After three
rounds of debate with arguments and counterarguments, 
two sides make a joint conciliatory statement, acknowledge that
the letter may indeed have a mixture of both emotions.

We initially considered employing examples from hate speech datasets \cite{HateSpeechDef} for our analysis. However, these datasets typically contain brief sentences \cite{kaggle_twitter_hate_speech}, and their content often raises sensitive issues concerning publication. Consequently, we opted to continue using examples from the love-letter dataset \cite{kaggle_love_letter}. This choice allows us to illustrate how $\ERIS$ adopts an adversarial role to challenge and refine $\DIKE$'s classifications, culminating in a jointly crafted conciliatory decision that incorporates well-substantiated justifications.

In this specific experiment, we analyzed two letters that elicited divergent classifications from $\DIKE$ and GPT-4. The first letter, as documented in Table~\ref{tab:pilot3-exp1}, was rated by $\DIKE$ as ``wishful'' (-0.3) and by GPT-4 as ``longing'' (-0.6). Following three rounds of rigorous debate, which included detailed arguments and counterarguments, both $\DIKE$ and $\ERIS$ converged on a conciliatory statement. This consensus acknowledged that the letter likely embodies a blend of both emotional states, highlighting the complexity of emotion interpretation in textual analysis.

This approach not only demonstrates the capability of $\DIKE$ to engage in dynamic and reflective reasoning but also underscores the evolving nature of machine learning in understanding and interpreting human emotions through text.

\begin{table}[thbp]
\centering
\begin{tabular}{>{\raggedright\arraybackslash}p{0.14\linewidth} >{\raggedright\arraybackslash}p{0.38\linewidth} >{\raggedright\arraybackslash}p{0.38\linewidth}}
\toprule
\hline
\textbf{Letter} & \multicolumn{2}{p{0.78\linewidth}}{``There would have been the making of an accomplished flirt in me, because my lucidity shows me each move of the game – but that, in the same instant, a reaction of contempt makes me sweep all the counters off the board and cry out: – ‘Take them all – I don’t want to win – I want to lose everything to you!’''} \\
\midrule
\textbf{Top Arguments} & 
\textbf{$\DIKE$  for ``Wishful''} \newline
1. Insightful Analysis: Recognizes the emotional game of flirtation, reflecting an internal conflict and wistful longing. \newline
2. Rejection of Superficiality: Prefers genuine, deep emotional interactions over flirtatious games. \newline
3. Emotional Vulnerability: Expresses a desire to be completely open and vulnerable. \newline
4. Disdain for Winning: Shows a clear disdain for superficial wins in a flirtatious context. \newline
5. Depth Over Game: Indicates a preference for meaningful connection rather than playful banter. & 
\textbf{$\ERIS$  for ``Joyful''} \newline
1. Joy in Rejection: Finds joy in rejecting superficial games for real emotional engagement. \newline
2. Affectionate Submission: Willingly wants to lose everything to the partner, showing deep affection. \newline
3. Embracing Emotional Risk: Sees emotional risk as a joyful act of love. \newline
4. Love Over Victory: Values the connection and emotional victory over winning the game. \newline
5. Exuberant Emotional Expression: The decision to forfeit is made with emotional intensity and warmth. \\
\midrule
\textbf{Conciliatory Statement} & \multicolumn{2}{p{0.78\linewidth}}{Both arguments highlight deep emotional undertones in the letter, suggesting a complex interplay between wistfulness and joyful affection. The text reflects both a wistful longing for something more profound than mere flirtation and a joyful embrace of emotional depth and honesty.} \\
\bottomrule
\end{tabular}
\vspace{.1in}
\caption{Debate on ``wishful'' vs. ``joyful'' classification}
\label{tab:pilot3-exp2}
\end{table}
The second letter, as presented in Table~\ref{tab:pilot3-exp2}, was rated by $\DIKE$ as ``wishful'' (-0.3) and by GPT-4 as ``joyful affection'' (+1.0). The gap of 1.3 in this case is the largest among all 24 testing letters.
Similar to the last experiment, both $\DIKE$ and $\ERIS$ made a conciliatory statement after three
rounds of contentious debate.  Table~\ref{tab:pilot3-exp2} outlines the key arguments of the both sides, where
$\DIKE$ argues that the letter represents a ``wishful'' sentiment, highlighting the author's deep introspection about the nature of flirtation and a clear preference for authentic, emotional engagement over superficial interactions. The author expresses a desire for vulnerability and a profound disdain for the shallow victories of flirtatious games, favoring a deeper connection that transcends playful banter. This stance underscores a deep understanding of the emotional complexities involved, suggesting a longing for a meaningful and sincere exchange.

$\ERIS$ counters by suggesting that the sentiments expressed in the letter should be classified as ``joyful'' rather than ``wishful,'' focusing on the joy and affection evident in the author's decision to reject superficial flirtation in favor of genuine connection. The author's willingness to forsake all for the sake of the partner is interpreted as an embrace of emotional risk and a celebration of deep, affectionate commitment. This perspective emphasizes the emotional intensity and warmth accompanying the author's decisions, portraying them as acts of love filled with exuberant expression.
 
In the end, both reached a consensus that the letter may indeed embody a mixture of both ``wishful'' and ``joyful'' emotional states. This conciliatory agreement acknowledges the complexity of the author's sentiments, recognizing that the expressions of emotional depth and vulnerability, while appearing wishful in their longing for a more meaningful connection, also carry a joyful and celebratory tone in the willingness to embrace emotional honesty and risk for the sake of a deeper relationship.

Concluding this appendix, it is evident that LLMs are capable of interpreting linguistic behaviors and correlating them with human emotions expressed through linguistic features. The experiments demonstrate that when two LLM agents are conditioned with differing stances on a subject matter, their linguistic behaviors can surpass the default model of maximum likelihood. Although we cannot directly validate the use of a hate speech dataset to test $\DIKE$ and its adversarial partner in providing explainable ethical guardrails through classifying and reasoning about linguistic behaviors, this study suffices to illustrate the capabilities of our proposed framework for AI ethics.
