# Supplementary material for: A Checks-and-Balances Framework for Context-Aware Ethical AI Alignment
Source: arXiv:2502.00136 source file (2025-05-28)
Supplement: Supplementary file 5 [file AppendixSystem1System2V01.tex]

\section{The $\UCCT$ Thesis: LLMs as the Unconscious Substrate for Intelligence}
\label{app:UCCT-theory}

This appendix addresses a key question: Why can a self-supervised pipeline, using only 54 rewritten love letters spanning diverse emotional behaviors, effectively instruct a Large Language Model (LLM) to perform emotion-behavior classification through few-shot prompting?

The \textit{Unconscious–Conscious Complementarity Thesis} ($\UCCT$), introduced in \textit{Multi-LLM Agent Collaborative Intelligence} \cite{AGIBookChang2024}, offers a layered theory of intelligence. It posits that LLMs function as an unconscious substrate, an immense self-supervised pattern-accumulating infrastructure, while few-shot interaction and real-world feedback instantiate a conscious layer that maps these latent patterns to explicit semantic concepts.

\subsection{The Nature of Unconscious Processing}

LLMs are trained using a next-token prediction objective over massive text corpora through self-supervised learning. Although the training data inherently contains semantic structure through human-written text, the model receives no explicit semantic labels or categories. Documents are processed as flat sequences of tokens: the model is never directly informed whether the content relates to physics, literature, or cooking. Through this process, LLMs internalize a vast latent space that encompasses syntax, idioms, conceptual regularities, and cross-domain structures, all without explicit semantic anchoring.

This crucially mirrors human perceptual development. Consider visual processing: from the lateral geniculate nucleus (LGN) through the primary visual cortex (V1–V4) to the infero-temporal cortex (IT), the human brain transforms raw sensory input into increasingly complex representations—edges, contours, textures, and eventually object features \cite{felleman1991distributed, grillspector2014neural}. Specifically, we do not have subjective access to these intermediate computations. We cannot consciously experience our V1 neurons detecting edges or our MT/V5 region computing motion vectors. These processes remain ``unconscious'' in the specific sense that they are inaccessible to subjective report or voluntary control \cite{kandel2013principles, dehaene2011consciousness}.

\subsection{The Threshold Crossing: From Pattern to Meaning}

The transition from unconscious processing to conscious awareness exhibits a distinctive discontinuity. Visual objects do not gradually fade into consciousness—they appear suddenly when sufficient evidence accumulates. This threshold-crossing phenomenon, while not literally quantum mechanical, shares the property of discrete state transitions. Similarly, in LLMs, the few-shot prompting process creates a sudden semantic bridge: patterns that existed implicitly in the network's weights become explicitly mapped to meaningful categories.

The human brain accomplishes this semantic assignment through minimal supervision. A child needs only a few labeled exposures to reliably categorize objects, emotions, or concepts \cite{carey1978acquiring, lake2015human}. Deeper structures like the hypothalamus and brainstem contribute emotional valence and motivational significance to these perceptual representations, transforming neutral patterns into meaningful experiences. This process, where vast unconscious computation meets minimal conscious labeling, is precisely what Chang \cite{AGIBookChang2024} identifies as the core mechanism that few-shot learning recapitulates in artificial systems.

\subsection{Implications for the Love Letter Experiment}

The effectiveness of 54 rewritten love letters in teaching emotion-behavior classification demonstrates this principle in action. The LLM's pre-trained weights already encode rich patterns about emotional expression, behavioral descriptions, and their statistical relationships, learned implicitly through exposure to countless human texts. The few-shot examples do not teach these patterns from scratch; rather, they provide semantic anchors that map pre-existing latent structures to explicit categories.

This framework offers a more parsimonious explanation than alternatives that require extensive supervised training or complex architectural modifications. Just as the visual system's unconscious computations become meaningful through minimal labeling, LLMs' vast pattern spaces become functionally intelligent through strategic few-shot guidance. The $\UCCT$ thesis thus provides both a theoretical foundation for understanding LLM capabilities and a practical framework for designing effective prompting strategies.

%%%%%%%  Thesis Preso Shikhar Murty
\begin{comment}
    
Part I
Tree-struction projections to check generalization?
ACL 2023
Part II: Interactions...
BAGEL 2024NNetNav

\end{comment}

\vspace{0.5em}
\noindent\textbf{Few-Shot Grounding as Conscious Semantics.} 
Just as a child can identify a cousin from a few labeled exposures, LLMs can generalize a semantic mapping from a handful of annotated examples. This is not because the few shots teach the model new structures, but because they \textit{activate and align} existing latent patterns with explicit meaning. Thus, few-shot prompting is not just task specification—it is the computational analog of conscious attention and labeling.

\subsection{Failure Modes: Pattern Absence, Not Architectural Flaws}

The $\UCCT$ framework offers a precise diagnosis for when LLMs fail at few-shot tasks. The failure occurs not because LLMs lack reasoning capabilities, but because the training data lacks pattern coverage for the task at hand. If no latent structure exists for a concept (e.g., subject matter A is absent from the training corpus), few-shot learning has no pattern base to map from—just as a child cannot recognize an animal species they've never seen.

This interpretation reframes the question of LLM “intelligence.” LLMs are not expected to reason like humans—they are not conscious agents. They are repositories of learned patterns. Whether an LLM is “good” or “bad” depends on whether it contains the patterns necessary for semantic anchoring. When it fails, the solution is data augmentation (e.g., domain-specific pretraining or retrieval augmentation), not a redesign of the architecture.

\subsection{Intelligence Emerges from Collaborative Conscious Layers}

The $\UCCT$ further argues that intelligence is not an intrinsic property of a single model, but an emergent capability arising from layered and interactive systems. Drawing from Hegel's \textit{Science of Logic}, \cite{AGIBookChang2024} emphasizes that the ``I'' lacks reality until it enters into interactions, interactions marked by effort, responsibility, temporality, and social coordination. An LLM alone is like a deck of cards; the rules of the game, strategies, and goals are established through external systems.

Thus, conscious-level intelligence involves:
\begin{itemize}
    \item Grounding latent patterns through minimal supervision (few-shot learning).
    \item Constructing agentic frameworks that regulate, critique, and adapt model outputs.
    \item Enabling interaction, dialogue, and collaborative inference among multiple models or human-AI teams.
\end{itemize}

This perspective motivates the design of layered systems, such as \textsc{MACI} (Multi-Agent Collaborative Intelligence), that build conscious functions atop the unconscious substrate provided by LLM. These scaffolds do not replace LLMs but enable them to serve as \emph{semantic engines} for adaptive, ethical, and human-aligned cognition.

\subsection{Novel Contributions of the $\UCCT$ Perspective}

The $\UCCT$ framework advances the current discourse around LLMs and AGI in several novel ways:

\begin{itemize}
    \item \textbf{Functional Layering of Cognition:} It establishes a precise mapping between LLM-based statistical pattern recognition and the unconscious substrate of cognition, contrasting with vague analogies like "System 1 vs. System 2."
    
    \item \textbf{Grounded Explanation of Few-Shot Learning:} It reframes few-shot prompting not as mini-finetuning or mere task formatting, but as conscious-level anchoring of latent, unconscious representations.

    \item \textbf{Failure Conditions Made Explicit:} Provides a clear diagnostic principle: failures arise when the unconscious layer lacks sufficient pattern coverage, not due to architectural limitations, thus directing attention to data-centric remedies (e.g., RAG, focused fine-tuning).
    
    \item \textbf{Interaction as the Genesis of Intelligence:} Drawing on Hegelian dialectics, it asserts that intelligence emerges not from individual models but from systems capable of purpose, coordination, and mutual adaptation, placing multi-agent interaction at the core of artificial general intelligence.
\end{itemize}

\subsection{Other Related Perspectives}

The debate over whether Large Language Models (LLMs) can achieve Artificial General Intelligence (AGI) divides the AI community into three camps: proponents who see scaling as sufficient, skeptics who identify fundamental limitations, and moderates who view LLMs as necessary but insufficient components.

\paragraph{Proponents: Scaling Toward AGI.}
Leaders like Sam Altman (OpenAI) and Demis Hassabis (Google DeepMind) argue that LLMs already exhibit AGI-like capabilities through emergent behaviors in reasoning and few-shot learning \cite{Brown2020language, Wei2022emergent}. They propose that continued scaling, combined with alignment techniques and tool integration, will bridge remaining gaps. Hassabis envisions LLMs as "core reasoning engines" within modular AGI architectures \cite{Hassabis2024AGIfuture}, while Altman suggests that effective fine-tuning can align LLM world models with reality \cite{Altman2021moores}.

\paragraph{Skeptics: Fundamental Deficiencies.}
Critics like Yann LeCun (Meta AI) and Gary Marcus contend that LLMs are sophisticated pattern matchers lacking true understanding. LeCun dismisses them as ``autocomplete'' systems without causal reasoning or embodied experience \cite{LeCun2022path, Heaven2022LeCunInterview}, advocating instead for world models that learn through environmental interaction. Marcus emphasizes the absence of symbol grounding and direct perception, arguing that genuine intelligence requires reasoning beyond statistical correlations \cite{Marcus2022horse, Marcus2020next}.

\paragraph{Middle Ground: LLMs as Foundation.}
An emerging consensus views LLMs as crucial but insufficient for AGI. This perspective supports hybrid architectures that augment LLMs with specialized modules for grounding, memory, multi-modal processing, and verifiable reasoning \cite{Yao2023react, Xu2023rewoo, Mialon2023augmented}. Such approaches position LLMs as powerful components within layered cognitive architectures rather than standalone intelligent systems.

\subsection{Conclusion: LLMs Are Not the Problem—They Are the Foundation}

Critiques that LLMs lack ``understanding'' miss the foundational role they play. LLMs, like the unconscious mind or the foundation of a house, are not meant to reason or interpret. They provide the substrate, accumulated through unsupervised exposure to vast patterns, upon which intelligent behavior can be constructed.

AGI, from the $\UCCT$ standpoint, is not the product of scaling alone. It is the product of aligning unconscious structure with conscious supervision and embedding both within collaborative architectures. What matters is not whether LLMs can think alone, but whether we can build systems that let them think \textit{together}.
