# Supplementary material for: A Checks-and-Balances Framework for Context-Aware Ethical AI Alignment
Source: arXiv:2502.00136 source file (2025-05-28)
Supplement: Supplementary file 6 [file AppendixSystem1System2V02.tex]

\section{The $\UCCT$ Thesis: LLMs as the Unconscious Substrate for Intelligence}
\label{app:UCCT-theory}

This appendix addresses a key question: Why can a self-supervised pipeline, using only 54 rewritten love letters spanning diverse emotional behaviors, effectively instruct a Large Language Model (LLM) to perform emotion-behavior classification through few-shot prompting?

The \textit{Unconscious–Conscious Complementarity Thesis} ($\UCCT$), introduced in \textit{Multi-LLM Agent Collaborative Intelligence} \cite{AGIBookChang2024}, offers a layered theory of intelligence. It posits that LLMs function as an unconscious substrate, an immense self-supervised pattern-accumulating infrastructure, while few-shot interaction and real-world feedback instantiate a conscious layer that maps these latent patterns to explicit semantic concepts.

\vspace{-0.1in}
\subsection{The Nature of Unconscious Processing}

LLMs are trained using a next-token prediction objective over massive text corpora through self-supervised learning. Although the training data inherently contains semantic structure through human-written text, the model receives no explicit semantic labels or categories. Documents are processed as flat sequences of tokens: the model is never directly informed whether the content relates to physics, literature, or cooking. Through this process, LLMs internalize a vast latent space that encompasses syntax, idioms, conceptual regularities, and cross-domain structures, all without explicit semantic anchoring.

This crucially mirrors human perceptual development. Consider visual processing: from the lateral geniculate nucleus (LGN) through the primary visual cortex (V1–V4) to the infero-temporal cortex (IT), the human brain transforms raw sensory input into increasingly complex representations—edges, contours, textures, and eventually object features \cite{felleman1991distributed, grillspector2014neural}. Specifically, we do not have subjective access to these intermediate computations. We cannot consciously experience our V1 neurons detecting edges or our MT/V5 region computing motion vectors. These processes remain ``unconscious'' in the specific sense that they are inaccessible to subjective report or voluntary control \cite{kandel2013principles, dehaene2011consciousness}.

\vspace{-0.1in}
\subsection{The Threshold Crossing: From Pattern to Meaning}

The transition from unconscious processing to conscious awareness exhibits a distinctive discontinuity. Visual objects do not gradually fade into consciousness—they appear suddenly when sufficient evidence accumulates. This threshold-crossing phenomenon, while not literally quantum mechanical, shares the property of discrete state transitions. One could relate this to physiological thresholds: dopamine release triggering reward recognition, or cardiac rhythms modulating attention states. Consciousness awakens when neural activation exceeds critical thresholds, analogous to how ReLU activation functions gate information flow in artificial networks. Similarly, in LLMs, the few-shot prompting process creates a sudden semantic bridge: patterns that existed implicitly in the network's weights become explicitly mapped to meaningful categories.

Our brain accomplishes this semantic assignment through minimal supervision. A child needs only a few labeled exposures to reliably categorize objects, emotions, or concepts \cite{carey1978acquiring, lake2015human}. Deeper structures such as the hypothalamus and brainstem contribute to emotional valence and motivational significance to these perceptual representations, transforming neutral patterns into meaningful experiences. This process, where vast unconscious computation meets minimal conscious labeling, is what \cite{AGIBookChang2024} identifies as the core mechanism that few-shot learning recapitulates in artificial systems.

%\vspace{-0.1in}
\subsection{Implications for the Love Letter Experiment}

The effectiveness of 54 rewritten love letters in teaching emotion-behavior classification demonstrates this principle in action. The LLM's pre-trained weights already encode rich patterns about emotional expression, behavioral descriptions, and their statistical relationships, learned implicitly through exposure to countless human texts. The few-shot examples do not teach these patterns from scratch; rather, they provide semantic anchors that map pre-existing latent structures to explicit semantics. Conceptually, similar patterns likely reside in proximate regions of the same manifold, allowing few-shot examples to activate entire neighborhoods of related representations.

This framework offers a more parsimonious explanation than alternatives that require extensive supervised training or complex architectural modifications. Just as the visual system's unconscious computations become meaningful through minimal labeling, LLMs' vast pattern spaces become functionally intelligent through strategic few-shot guidance. Thus, the thesis $\UCCT$ provides both a theoretical foundation for understanding the capabilities of LLM and a practical framework for designing effective prompting strategies.

%\vspace{-0.1in}
\noindent\textbf{Few-Shot Grounding as Conscious Semantics.} 
Just as a child can identify a cat from a few labeled exposures, LLMs can generalize a semantic mapping from a handful of annotated examples. This is not because the few shots teach the model new structures, but because they \textit{activate and align} existing latent patterns with explicit meaning. Thus, a few-shot prompting is not just a task specification; it is the computational analog of conscious attention and labeling.

%\vspace{-0.1in}
\subsection{Failure Modes: Pattern Absence, Not LLM Flaws}

The $\UCCT$ framework offers a precise diagnosis for when LLMs fail at few-shot tasks. The failure occurs not because LLMs lack reasoning capabilities, but because the training data lacks pattern coverage for the task at hand. If no latent structure exists for a concept (e.g., a specialized domain absent from the training corpus), few-shot learning has no pattern base to map from—just as a child cannot recognize an animal species they've never encountered in any form. 

This interpretation reframes the question of LLM ``intelligence.'' LLMs are not expected to reason like humans—they are not conscious agents. They are repositories of learned patterns. Whether an LLM succeeds or fails depends on whether it contains the patterns necessary for semantic anchoring. When it fails, the solution is data augmentation (e.g., domain-specific pretraining or retrieval augmentation), not architectural redesign.

%%%%%%%

\subsection{Intelligence Emerges from Multi-LLM Interaction and Collaboration}

Building upon this foundation, we can hypothesize a pathway to more advanced intellectual capabilities through multi-LLM collaboration. Drawing metaphorically from Hegelian dialectics, a system where two or more LLMs engage in moderated interaction could achieve a higher order of semantic grounding'' and reasoning. If such interactions are structured to foster contentiousness'', allowing differing perspectives or outputs (a thesis and its antithesis) to emerge and are driven by an engineered impetus for engagement and resolution (akin to ``module desire'' fueled by rewards), the system could be guided towards a richer synthesis. This synthesized understanding, emerging from the dynamic interplay and resolution of differences, would ideally transcend the capabilities of any individual LLM operating in isolation, reflecting Hegel's insight that progress and deeper truth often arise from the productive struggle with negation and the integration of diverse viewpoints. This framework, while an analogy, suggests that appropriately structured multi-agent contention and collaboration, underpinned by the $\UCCT$, could be a key to unlocking more sophisticated emergent intelligence.

Indeed, this emphasis on interaction aligns with the core of the $\UCCT$, which posits that intelligence is not an intrinsic property of a single model but an emergent capability arising from layered and interactive systems. Such a perspective resonates with deeper philosophical insights; for instance, Chang \cite{AGIBookChang2024}, drawing from Hegel's \textit{Science of Logic}, emphasizes that the "I" (as a realized form of being or intelligence) lacks substantive reality until it enters into interactions marked by effort, responsibility, temporality, and social coordination. In this light, an LLM alone is like a deck of cards; the game itself, its rules, strategies, and goals, is only established through external interactive systems that orchestrate its participation, potentially in concert with other agents. Further discussion on the specifics of multi-LLM collaborative intelligence is beyond the scope of this paper.

\subsection{Conclusion: LLMs Are Not the Problem—They Are the Foundation}

Critiques that LLMs lack ``understanding'' miss the foundational role they play. LLMs, like the unconscious mind or the foundation of a house, are not meant to reason or interpret. They provide the substrate, accumulated through self-supervised exposure to vast patterns, on which intelligent behavior can be constructed.

AGI, from the $\UCCT$ standpoint, is not the product of scaling alone. It is the product of aligning unconscious structure with conscious supervision and embedding both within collaborative architectures. What matters is not whether LLMs can think alone, but whether we can build systems that let them think \textit{together}.
